# Supplementary material for: Lower Bounds for Differential Privacy from Gaussian Width
Source: arXiv:1612.02914 source file (2016-12-09)
Supplement: Supplementary file 1 [file appendix2.tex]

\section{Sample Complexity Proofs}
\label{app:sample}

Below we include the omitted proofs of the sample complexity
properties introduced in Section~\ref{sec:bp}.

%\begin{lemma}\label{lemma:subsetsc}
%$L \subseteq K \Rightarrow \forall \alpha \in (0,1): \scz(L,\alpha)
%\leq \scz(K,\alpha)$  
%\end{lemma}

%\begin{corr}\label{b2bound}
%For all $\epz = O(1)$, $2^{-\Omega(n)} \leq \delta \leq 1/n^{1 +
%  \Omega{(1})}$ and $\alpha \leq 1/10$: 
%\[\scz(B_2^m, \alpha) = \Omega{\left( \frac{\sqrt{m \log{1/\delta}}}{\alpha \epz} \right)}.\]
%\end{corr}

%\begin{proof}[Proof of Corollary~\ref{b2bound}]
%Since $Q^m \subseteq B_2^m$, this follows directly from
%\autoref{lemma:subsetsc} and \autoref{thm:tightcube}.
%\end{proof}

% \begin{lemma}\label{lemma:linop2}
%   For any $\alpha \in (0,1)$, any linear operator $T \maps
%   \R^m \rightarrow \R^m$ and any symmetric convex body
%   $K \subset \mathbb{R}^m$: $$ \scz(K, \alpha) \geq \scz( T(K), \alpha
%   \cdot \|T\|).$$
% \end{lemma}

% \begin{corr}\label{scaling}
%   For any $t > 0$: \[ \scz(tK, t\alpha) = \scz(K, \alpha).\]
% \end{corr}

% \begin{theorem}[Geometric Lower Bound]{\label{modularlb}}
%   For all $\epz = O(1)$, $2^{-\Omega(n)} \leq \delta \leq 1/n^{1 +
%     \Omega{(1})}$, any convex symmetric body $K \subseteq
%   \mathbb{R}^m$, any $1 \le k \le m$ and any $\alpha \le
%   1/(10c_{k}(K^\circ))$: 
  
%   \[
%   \scz(K, \alpha) 
%   = \Omega \left(
%     \frac{\sqrt{\log{1/\delta}}}{\alpha \epz} 
%     \cdot \frac{\sqrt{m - k + 1}}{c_k(K^\circ)}
%   \right).
%   \]
%  \end{theorem}

\section{Arbitrary Body Lower Bounds}
\label{app:arbitrary}

\section{Mean Point to Query Release}
\label{app:meanpt}

Below we provide the complete reduction between the Mean Point problem and Query release, along with the relevant proofs.
